# Supplementary material for: TURNER: The Uncertainty-based Retrieval Framework for Chinese NER
Source: arXiv:2202.09022 source file (2022-02-18)
Supplement: Supplementary file 1 [file appendix.tex]

\typeout{IJCAI--22 Instructions for Authors}

% These are the instructions for authors for IJCAI-22.

\documentclass{article}
\pdfpagewidth=8.5in
\pdfpageheight=11in
% The file ijcai22.sty is NOT the same as previous years'
\usepackage{ijcai22}

% Use the postscript times font!
\usepackage{times}
\usepackage{soul}
\usepackage{url}
\usepackage[hidelinks]{hyperref}
\usepackage[utf8]{inputenc}
\usepackage[small]{caption}
\usepackage{graphicx}
\usepackage{amsmath}
\usepackage{amsthm}
\usepackage{booktabs}
\usepackage{algorithm}
\usepackage{algorithmic}
\usepackage{float}
\usepackage{mathtools}
\usepackage{multirow}
\usepackage{CJKutf8}
\usepackage{color}
\usepackage[T1]{fontenc}
\urlstyle{same}

% template and that you must *not* alter the styling.

% PDF Info Is REQUIRED.
% Please **do not** include Title and Author information
\pdfinfo{
/TemplateVersion (IJCAI.2022.0)
}

\begin{document}

\end{document}
